# Supplementary material for: Fine-Tuned Large Language Model for Visualization System: A Study on Self-Regulated Learning in Education
Source: arXiv:2407.20570 source file (2024-07-30)
Supplement: Supplementary file 1 [file 9-appendix.tex]

\section*{Supplementary Materials}
% The collection of supplementary materials is provided to enhance understanding and facilitate the evaluation of our work. It encompasses:

% % \begin{itemize}
% \textbf{Supplementary Material for Fine-tuning Process} elaborates on the methodologies employed in data processing, construction, model fine-tuning, and evaluation, offering insights into the technical foundations of our work.
% \textbf{Supplementary Material for Model Performance} contains the datasets used for testing the fine-tuned model, along with results obtained from multiple tests across different models. 
% \textbf{Supplementary Material for User Study} offers the presentation of the user study protocol, including an introduction to the evaluation metrics and a detailed exposition of the experimental results.

% \textbf{Video Material} facilitates a deeper and more intuitive understanding of Tailor-Mind and our efforts. 
% % \end{itemize}
